# Supplementary material for: CircuitVAE: Efficient and Scalable Latent Circuit Optimization
Source: arXiv:2406.09535 source file (2024-06-13)
Supplement: Supplementary file 1 [file appendix.tex]

\section{Appendix}

\input{sections/background}
\input{sections/related}

\subsection{Dataset}
We release a dataset of circuits designed by CircuitVAE, together with their latent representations and simulation results.
This dataset would be appropriate for reproducing the figures in this work, developing methods that predict circuit properties,  and analyzing the latent circuit representations that CircuitVAE learns. 
The dataset format is documented in \autoref{table:ds_columns}.

Due to the file size and anonymity constraints of the NeurIPS supplement, we only release data from one experiment at this time.
This experiment contains 64-bit adders designed by CircuitVAE with a delay weight of 0.95, a starting dataset of 30 GA generations, and a random seed of 1.
Following de-anonymization, we will release all the remaining data.

\begin{table}[h]
  \caption{Format of released data}
  \vspace{0.5em}
  \centering
  \begin{tabular}{ll}
    \toprule
    Column & Description \\
    \midrule
    \texttt{index} & Number of syntheses before this circuit \\
    \texttt{outer\_loop} & Round of training and optimization this circuit came from \\
    \texttt{step} & Gradient step of optimization this circuit was synthesized at \\
    \texttt{batch\_idx} & Which latent trajectory in the batch this circuit belonged to \\
    \texttt{bitvector} & The circuit's prefix graph, represented as a bitvector \\ & (see \autoref{subsec:synthesis}) \\ 
    \texttt{latent} & CircuitVAE's latent encoding of this circuit, a 128-vector \\
    \texttt{prior\_logprob} & The log-probability of this latent under the variational prior \\
    \texttt{true\_score} & The circuit's cost according to OpenPhySyn at this delay weight \\
    \texttt{predicted\_score} & The circuit's cost as predicted by CircuitVAE's cost predictor \\
    \bottomrule
  \end{tabular}
  \label{table:ds_columns}
\end{table}

\subsection{Circuit synthesis}
\label{subsec:synthesis}

In this section, we continue our discussion of the circuit synthesis flow used in this work in more detail.

Prefix graphs compactly represent a circuit's design in terms of carry \emph{generation} and \emph{propagation} \cite{bk}.
Each bit span \texttt{i:j} is associated with a generate bit $g_{i,j}$ and a propagate bit $p_{i,j}$.
For all $i=1 \ldots N$, computing the input bits $g_{i,i}$ and $p_{i,i}$ is straightforward; furthermore, given the output bits $(g_{1,1}; p_{1,1}) \ldots (g_{N,1}, p_{N,1})$, computing the final carries and summand is easy.
Intermediate values may be computed recursively: $(g_{i, j}; p_{i,j}) = (g_{i, x}; p_{i,x}) \circ (g_{x-1, j}; p_{x-1,j})$ where $i \geq x > j$ and $\circ$ is the carry operator Brent and Kung describe.
A prefix graph is exactly a tree determining the association order of $(g_{i,i}; p_{i,i}) \circ \ldots \circ (g_{1,1}; p_{1,1})$ for each $i = 1, \ldots, N$.

In the dataset we release, we compactly represent prefix graphs as \emph{bitvectors} with one bit per possible node in the graph.
For input to our CNN encoder, we reshape the bitvector into a matrix in $\{0, 1\}^{N \times N}$ where the upper triangular holds the bitvector values and the lower triangular holds zeroes; the CNN decoder predicts logits of this shape, and we extract the upper triangular to predict a bitvector.
We found that this representation approximately colocates bits which are closely connected.

Before synthesizing a predicted bitvector, any missing nodes implied by parentless child nodes are inserted in a process we refer to as \emph{legalization}.
By legalizing before scoring vectors, our cost predictor effectively sees legalization as part of the cost function, and does not need to separately learn which vectors are valid.

A prefix graph may be converted into a circuit netlist and synthesized at a particular clock target to determine its area and delay.
Because of decisions made within the synthesis tool, a given circuit may achieve a range of areas and delays when synthesized at different clock targets.
In practice, we first synthesized each circuit with clock targets 0.0ns and 10.0ns to determine upper and lower bounds on achievable delay, and then synthesize twice more at clock targets linearly interpolated 4\% and 36\% between these bounds.
We then fit a cubic interpolator to these four (area, delay) tuples to predict the full curve of area and delay, and score the circuit based on the minimum cost along this curve according to our given delay weight.
We found this scheme predicted synthesis results almost perfectly at much lower cost than computing the entire curve, so we benchmarked all methods in this way.

\subsection{Model architecture and hyperparameters}
\label{subsec:model}
In this section, we document CircuitVAE's model architecture.
All search, training, and model hyperparameters are listed in \autoref{table:hparams}.

CircuitVAE uses a fully-convolutional encoder and decoder, with linear layers to map to and from the 128-dimensional latent space.
Each trunk consists of four residual blocks, each having two 5x5 convolutions; these sizes were picked to give output units a full receptive field.
We use GELU \cite{DBLP:journals/corr/HendrycksG16} as the activation function and do not use batch or layer normalization.
The latent space uses a diagonal unit normal prior.
The cost predictor is an MLP on top of the latent vector, with one hidden layer of 32 units, followed by GELU and a linear scalar predictor.
The encoder and decoder each have approximately 1M parameters, and the score predictor has about 4000.
The input to the encoder is a bitmatrix as described in \autoref{subsec:synthesis}, augmented with binary positional encodings indicating the location of input and output nodes.

\begin{table}[H]
  \caption{Hyperparameters}
  \vspace{0.5em}
  \centering
  \begin{tabular}{lll}
    \toprule
    Parameter & Value & Description \\
    \midrule
    \textbf{Experimental} & & \\
    Bitwidth &  16, 32, 64 & Sizes of circuits designed \\
    Delay weight & 0.33, 0.66, 0.95 & Sensitivity of objective to delay vs area \\
    GA generations & 1, 5, 10, 30 & Number of GA generations used as initial data \\
    \midrule
    \textbf{Search} & & \\
    Steps & 600 & Total latent gradient steps \\
    Synthesis period & 100 & Gradient steps between synthesizing circuits \\
    Batch size & 96 & Number of parallel latent trajectories per search \\
    $\gamma$ & 0.01 - 0.1 & Strength of prior regularization \\
    Learning rate & 0.1 & \\
    \midrule
    \textbf{Training} & & \\
    Search period & 5000 & Training steps between latent optimization rounds \\
    Batch size & 64 & \\
    Learning rate & 0.0002 & \\
    Gradient clipping & 1.0 & \\
    Gradient skipping & 400.0 & Skip updates with pre-clip gradient norm $\geq$ 400.0 \\
    AE loss weight & 0.03 & Weight of autoencoding term in $\beta$-VAE loss \\
    $\beta$ & 0.01 & Weight of KL term in $\beta$-VAE loss \\
    $\lambda$ & 10.0 & Weight of cost prediction loss \\
    KL warmup & 2000 & Steps to linearly warmup KL loss from 0 \\
    k & 0.001 & Data reweighting coefficient \\
    \midrule
    \textbf{Model} & & \\
    Latent dimension & 128 & \\
    CNN filters & 64 & \\
    CNN kernel size & 5 & \\
    CNN blocks & 4 & ResNetV2 residual blocks per encoder and decoder \\ 
    $f_\pi$ depth & 1 & Hidden layers in cost predictor \\
    $f_\pi$ width & 32 & Width of cost predictor hidden layers \\
    \bottomrule
  \end{tabular}
  \label{table:hparams}
\end{table}

\subsection{Ablations}
\label{subsec:ablations}

\begin{figure}%
    \centering
    \subfloat{{\includegraphics[width=0.475\textwidth]{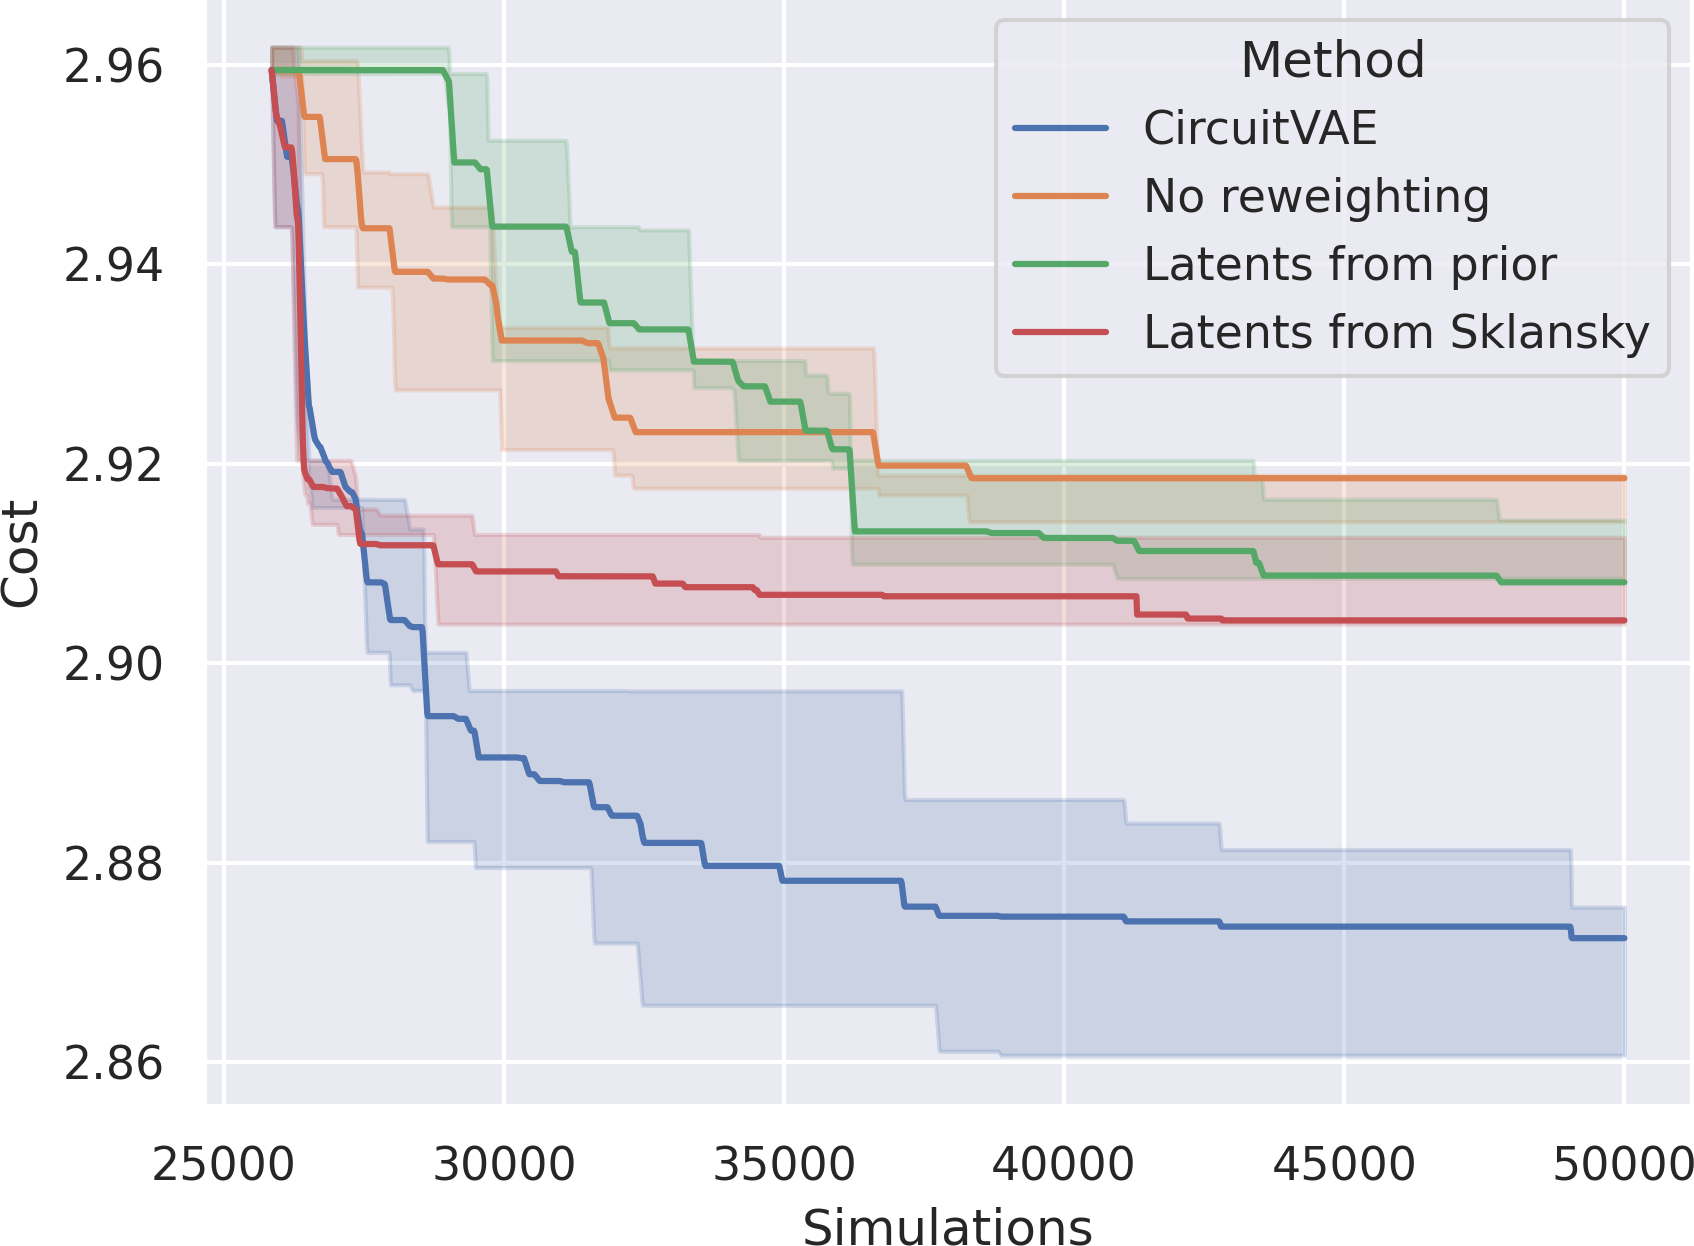} }}%
    \subfloat{{\includegraphics[width=0.475\textwidth]{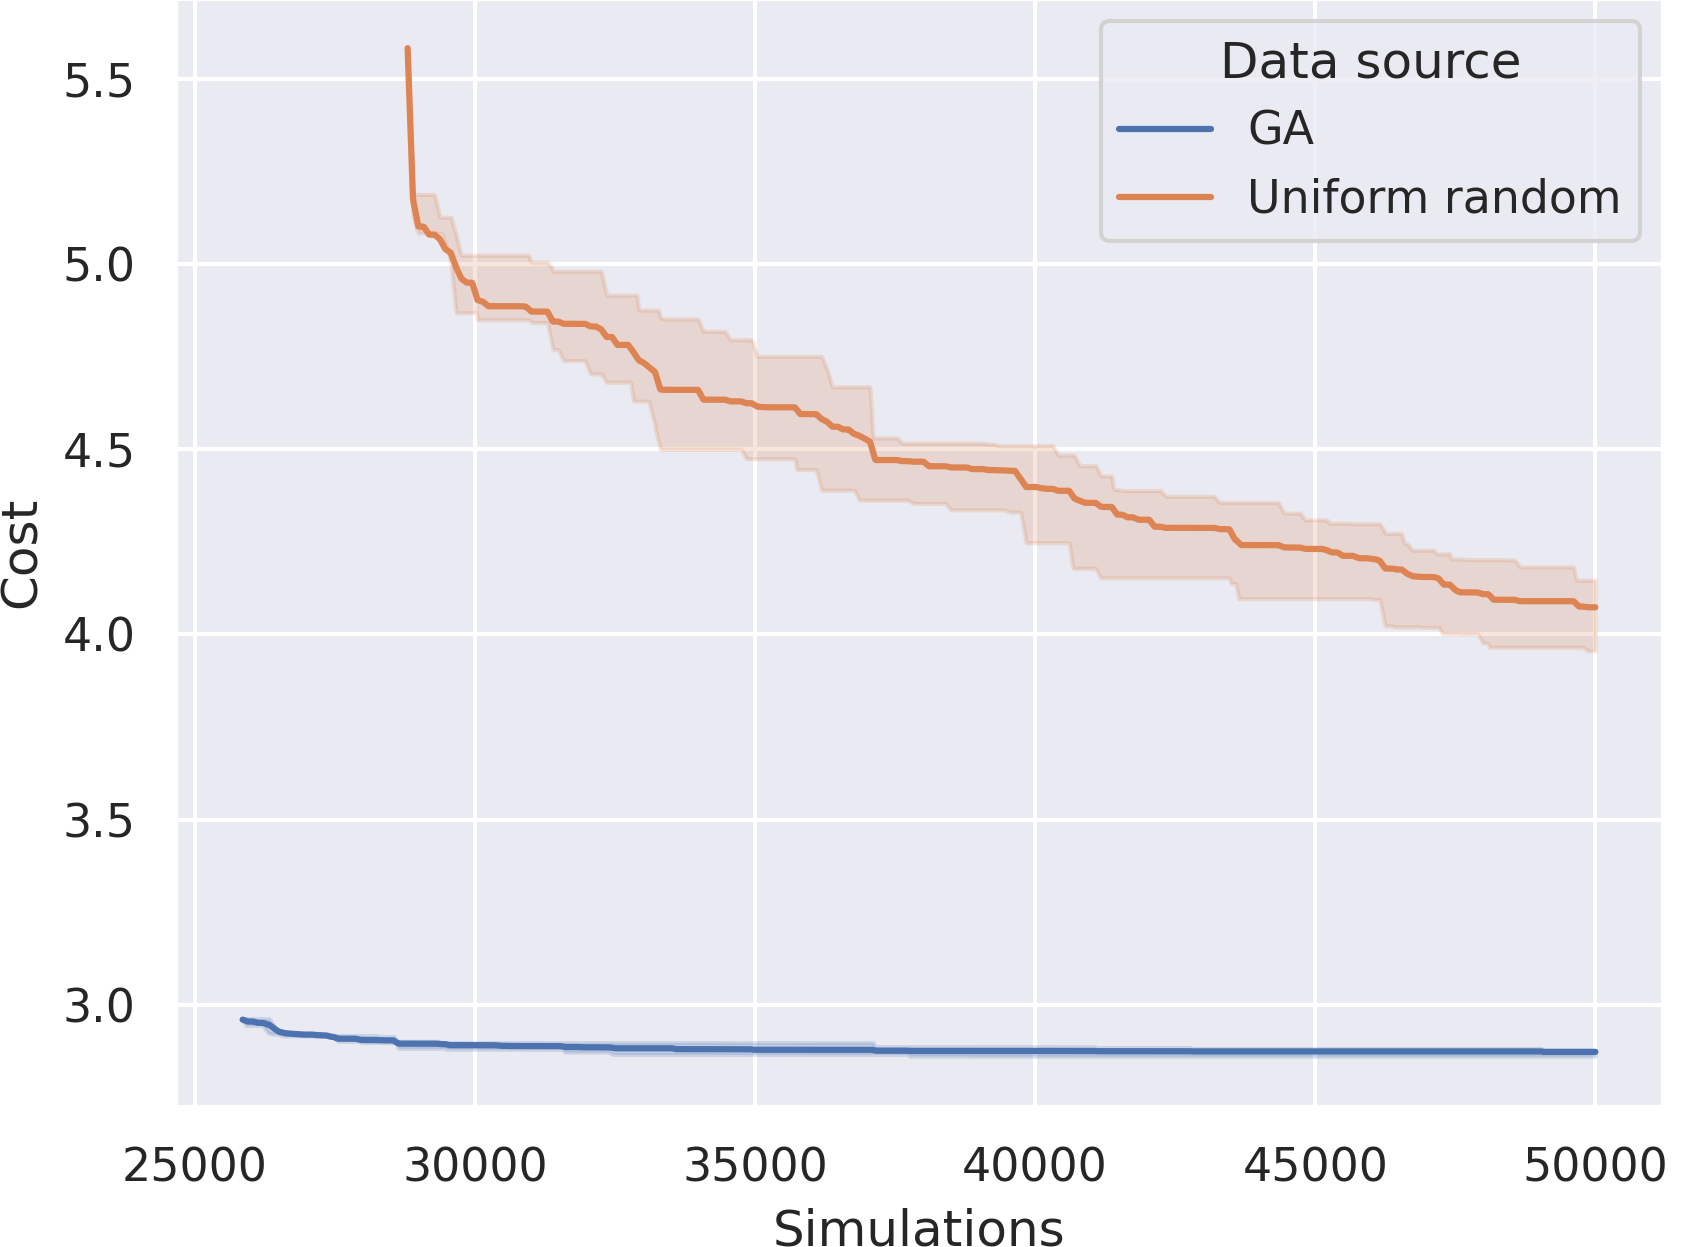} }}%
    \caption{Ablating search and training methods (left) and data source (right).}%
    \label{fig:abl_curves}%
\end{figure}

We ablated each of the components of CircuitVAE to understand their individual contributions.
All of these experiments were conducted on 32-bit adders, with a delay weight of 0.66 and the largest initial dataset.
In \autoref{fig:abl_curves}, we tested:
\begin{itemize}
    \item Removing data reweighting \citep{tripp2020sample}, which leads training to get stuck when new datapoints have a negligible impact on the overall distribution.
    \item Replacing the cost-weighted latent distribution with the prior or the latent encoding of Sklansky. Starting the search from a good adder (Sklansky) outperforms sampling from the prior, but both underperform our adaptive initialization. 
    \item Replacing the initial dataset with uniformly random adders rather than the first 30 generations of GA, which performs poorly because uniformly random adders are typically low-quality.  
\end{itemize}

\begin{figure}%
    \centering
    \subfloat{{\includegraphics[width=0.475\textwidth]{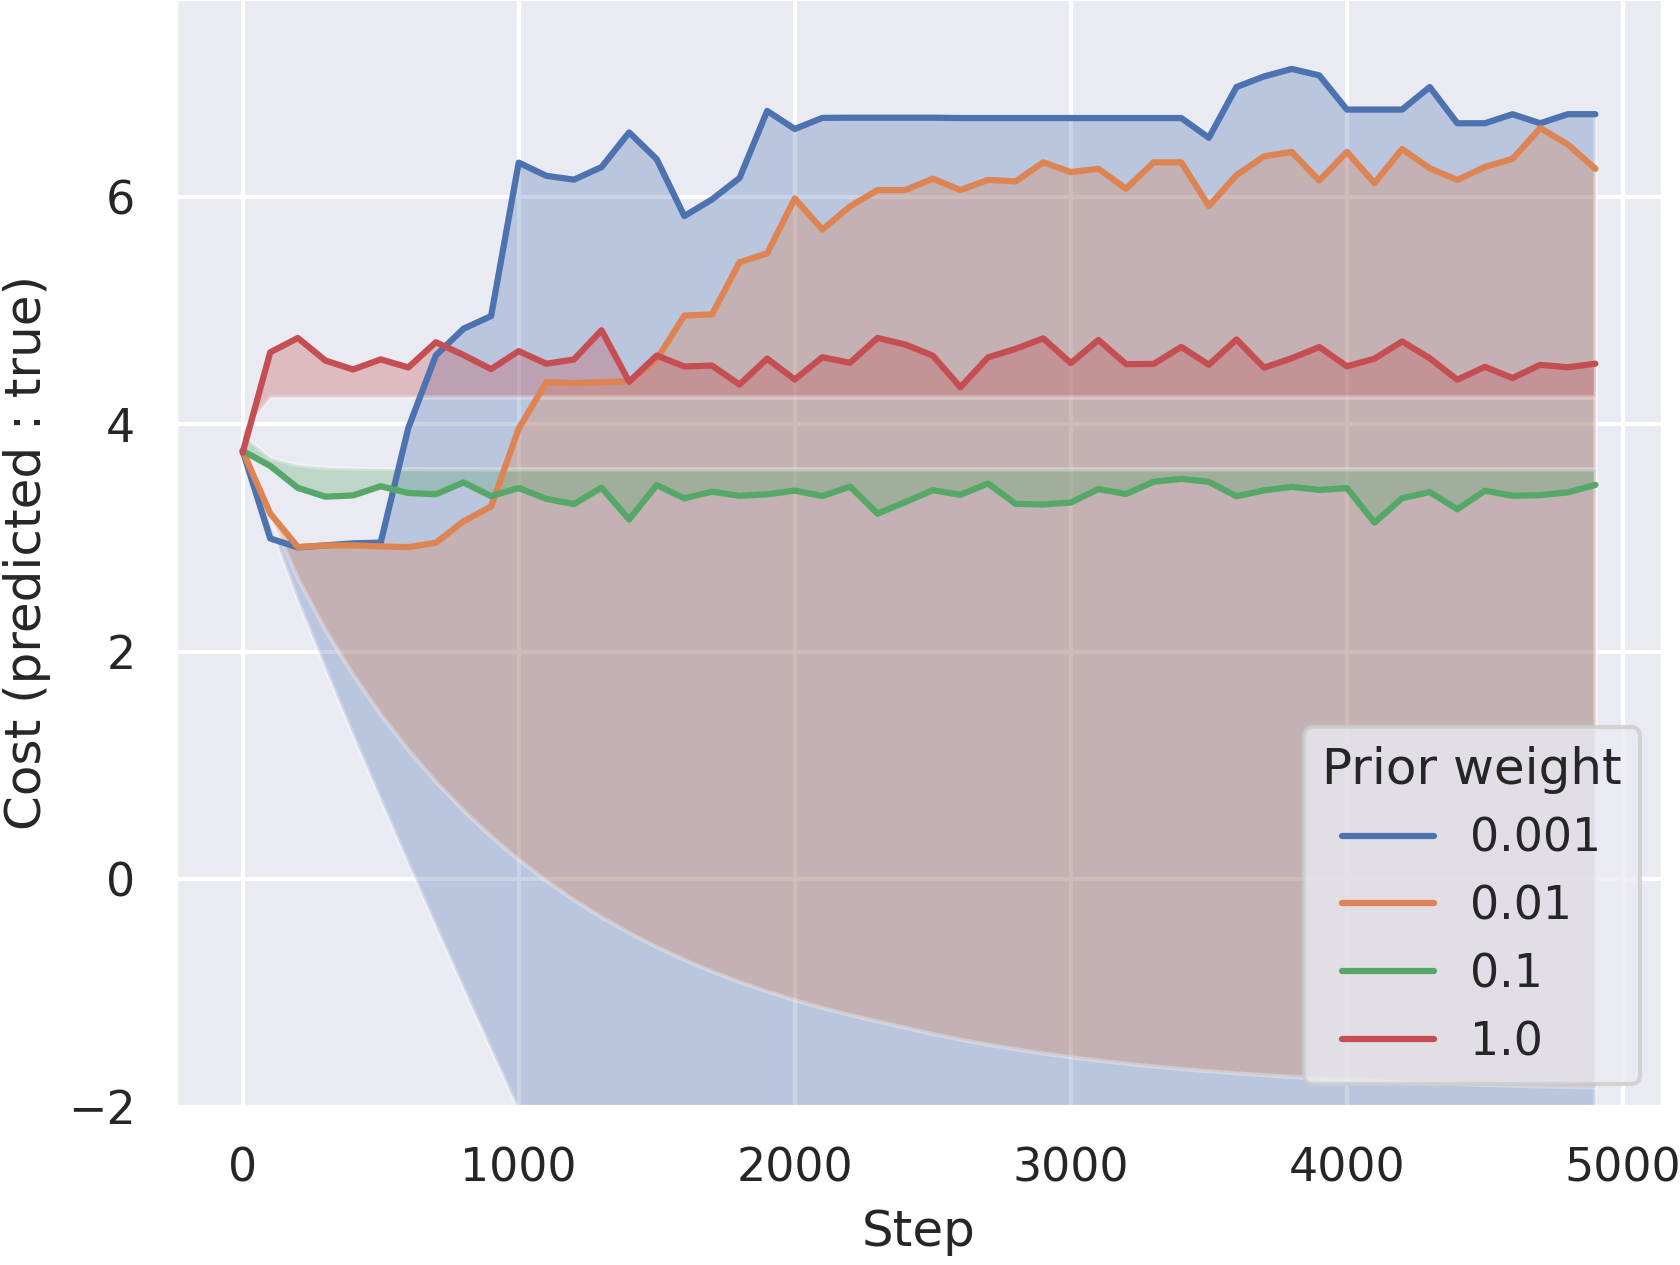} }} 
    \subfloat{{\includegraphics[width=0.475\textwidth]{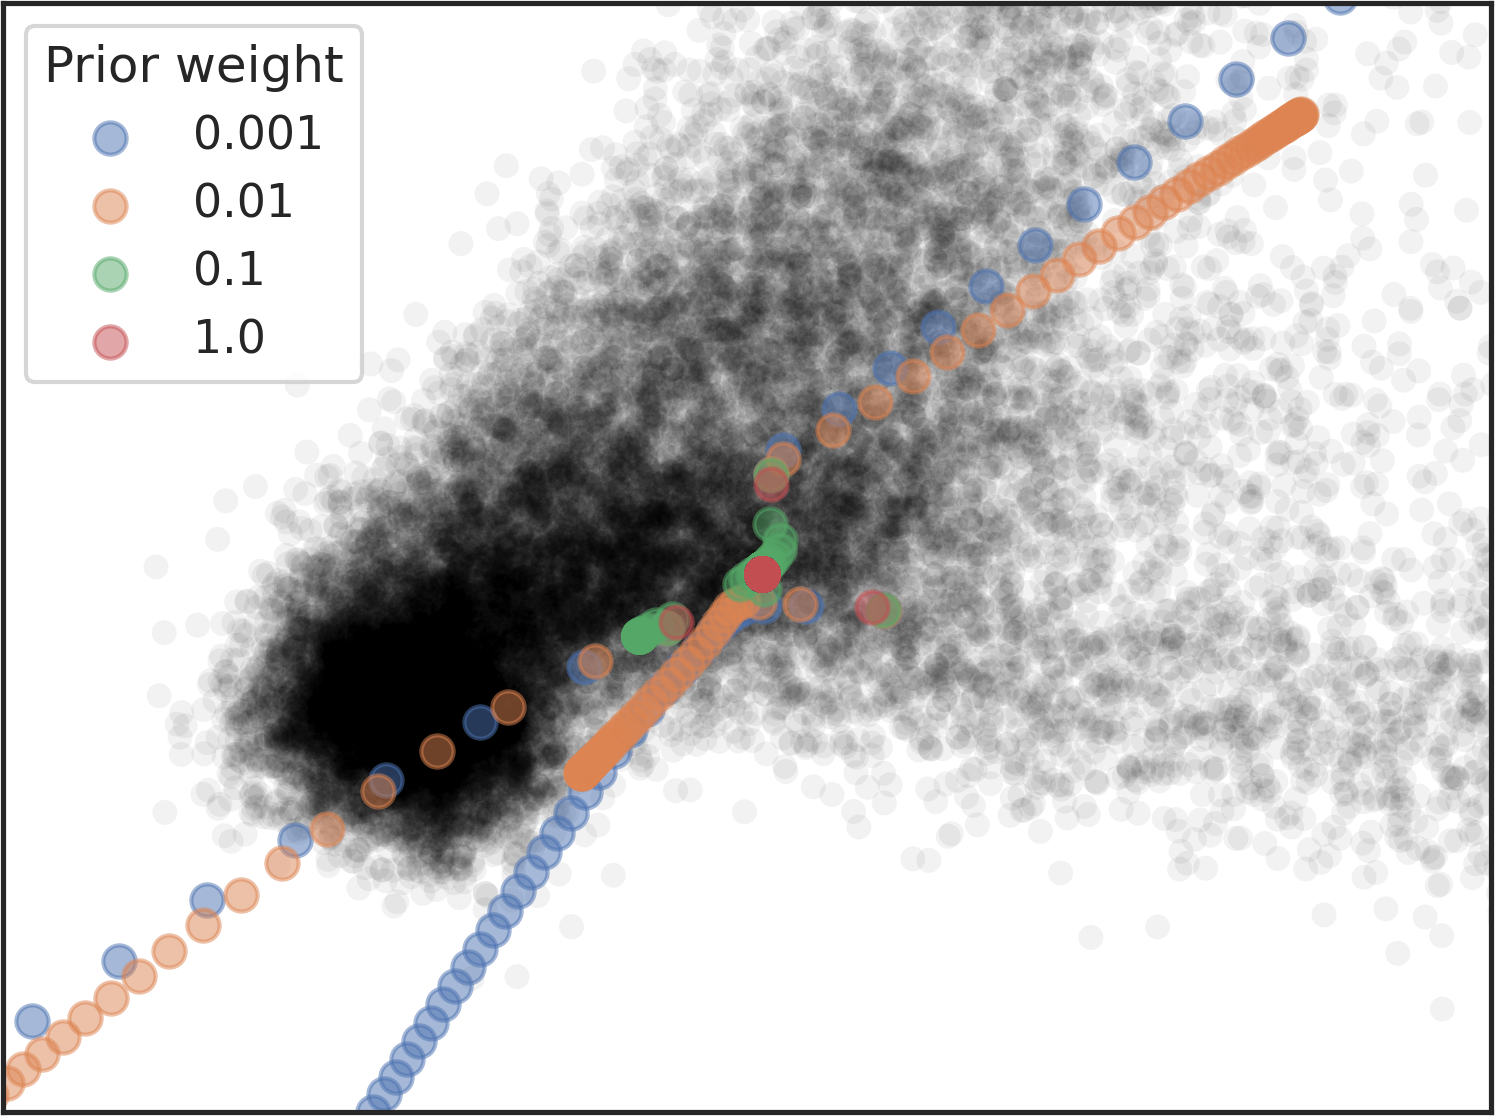} }}%
    \caption{The effect of changing prior weight $\gamma$ on cost (left) and latent search trajectories (right). Shaded regions show overfitting when the true cost (top) exceeds the model's prediction (bottom).}%
    \label{fig:abl_priorweight}%
\end{figure}

In \autoref{fig:abl_priorweight}, we examined the ability to control search by controlling the prior regularization term $\gamma$.
At low values of $\gamma$ (blue and orange), latent trajectories quickly exit the region around the training data (gray) and overfit the cost predictor, yielding much higher costs than the model predicts.
At higher values (green and red), trajectories stay near the origin, which prevents overfitting but limits exploration and sample diversity.
We found the best results from sampling values of $\gamma$ per latent trajectory log-uniformly between 0.01 and 0.1, and used this setting for all other experiments.

\subsection{Analyzing CircuitVAE's latent space}
\label{subsec:latent_analysis}

\begin{figure}
    \centering
    \includegraphics[width=\textwidth]{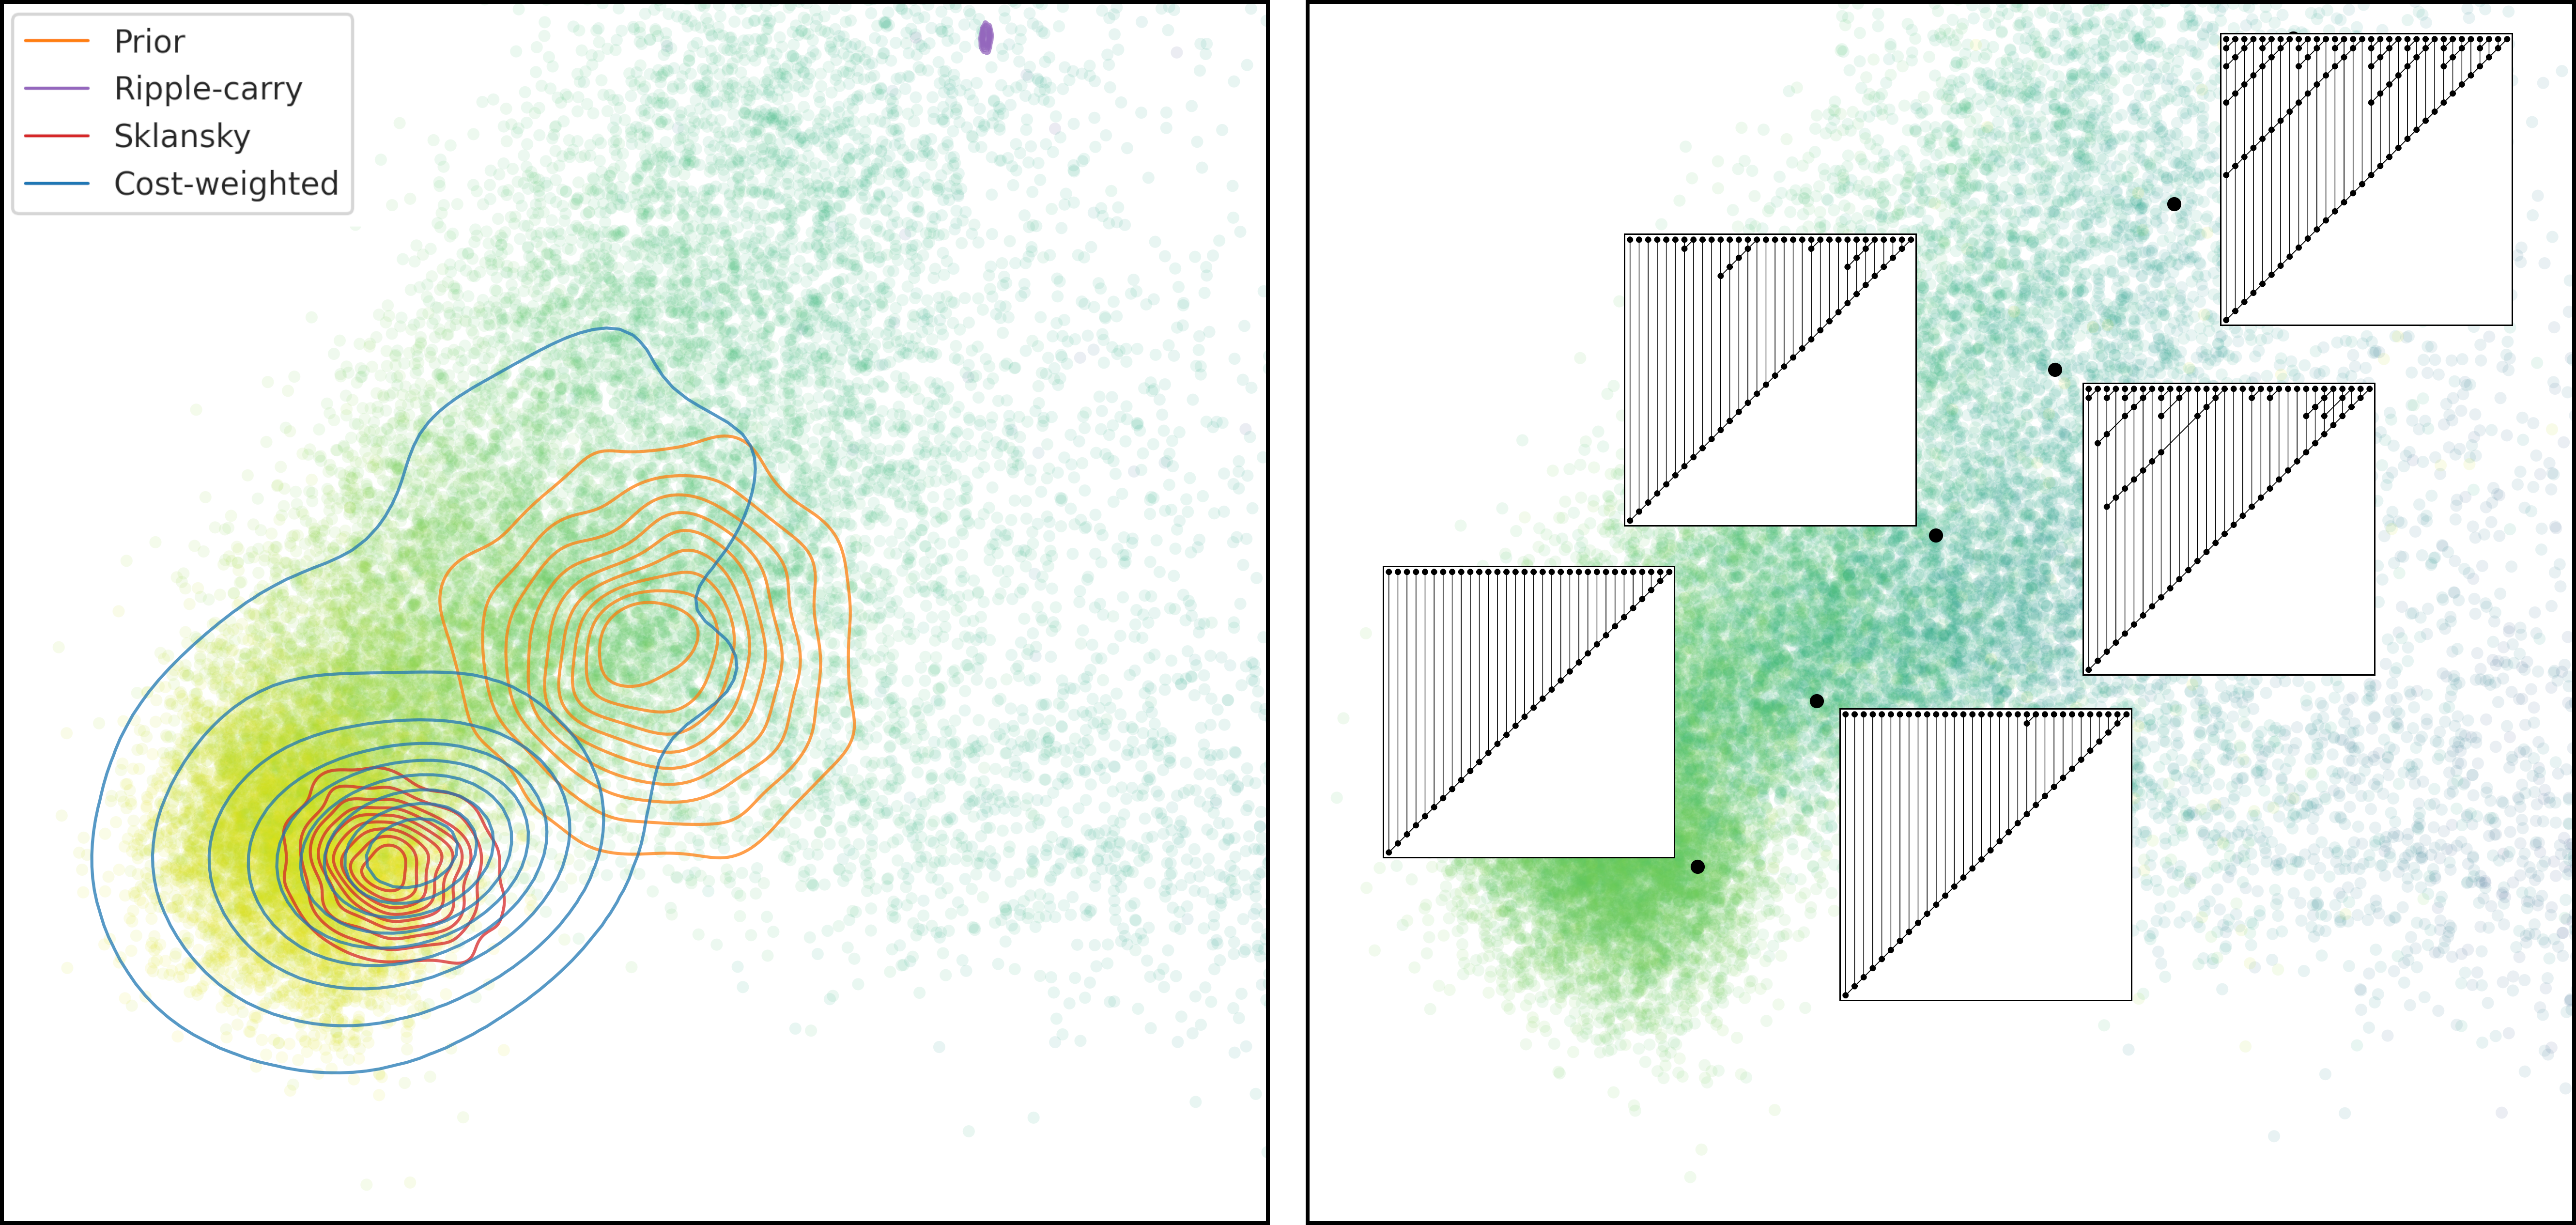}
    \caption{Left: Kernel density estimate plots of latent distributions. Right: interpolating between two circuits. Background points are training set adders, colored by cost (left) and area (right); lighter is better.}
    \label{fig:latent_regions}%
\end{figure}

To investigate properties of CircuitVAE's learned search space, we visualize it in two dimensions in \autoref{fig:latent_regions}.
We reduced 128-dimensional latent vectors down to two dimensions with PCA trained on encodings of training set points, and visualized dataset points and selected circuits in this space.

When the points are colored by cost (left) or area (right), it is clear that the latent space is self-organized according to both the objective function and physical properties of the circuits.
This is in stark contrast to the input space: represented as discrete graphs, nearby circuits (defined by having many nodes in common) may have very different costs and physical properties, since adding a single node may change the critical path.
While discrete search methods like GA and RL suffer from this poorly-structured search space, CircuitVAE learns its own space in which optimization is easy.

Visualizing different latent distributions (left) illustrates the benefits of our cost-weighted sampling approach.
Latents sampled from the prior are diverse but have subpar cost, while latents sampled from the posterior of specific circuits (ripple-carry and Sklansky) are typically higher quality but much less diverse.
Our cost-weighted distribution is diverse, covering much of the latent space, but is biased towards lower-cost adders.

% TODO

\subsection{GA baseline}
Our genetic algorithm (GA) baseline used a standard genetic algorithm with crossover and mutation operations \cite{davis1991handbook}. We used a population size of 1000 for each generation. The individuals of the population were the bitvector representations of flattened prefix graphs with each bit representing whether or not a prefix node was present. A single mutation was represented by a random inversion of a single Boolean value. Each individual was initialized by randomly choosing either the ripple-carry or Sklansky prefix structure and performing 200 random mutations. We assigned each individual a fitness score as negative cost as described in \autoref{subsec:synthesis}. Each successive generation was generated by taking the top 50\% most fit individuals from the previous generation and from them generating a new population. The new population was generated 40\% by a mutation procedure, 40\% by a crossover procedure, 10\% by preserving the top individuals from the previous generation unchanged and 10\% by the random initialization procedure mentioned above. The mutation procedure created a new individual by randomly sampling a single parent and then performing up to 50 random mutations. The crossover procedure created a new individual by randomly sampling two parents and then randomly choosing one of those two parents to supply the value at each node location.
